# Supplementary material for: Fluidization and wall slip of soft-glassy materials by controlled surface roughness
Source: arXiv:1611.01980 ancillary file (2016-11-07)
Supplement: Supplementary file 1 [file paper-supmat.pdf]

# Fluidization and wall slip of soft-glassy materials by controlled surface roughness: Electronic Supplementary Information (ESI)

Ladislav Derzsi,[1,*] Daniele Filippi,[1] Giampaolo Mistura,[1] Matteo Pierno,[1,†]
Matteo Lulli,[2] Mauro Sbragaglia,[2,‡] Massimo Bernaschi,[3] and Piotr Garstecki[4]

[1] *Dipartimento di Fisica e Astronomia "G. Galilei" - DFA and Sezione CNISM, Università di Padova, Via Marzolo 8, 35131 Padova, Italy*

[2] *Dipartimento di Fisica, Università di Roma "Tor Vergata" and INFN, Via della Ricerca Scientifica, 1 - 00133 Roma, Italy*

[3] *Istituto per le Applicazioni del Calcolo CNR, Via dei Taurini, 9 - 00185 Roma, Italy*

[4] *Institute of Physical Chemistry, Polish Academy of Sciences, Kasprzaka 44/52, 01-224 Warsaw, Poland*

(Dated: November 7, 2016)

## I. EXPERIMENTS

**Fabrication of microchannels:** The microfluidic channels were fabricated with a standard multilayer photolithographic technique: in the first step we spincoated a thin ($\simeq 2$ $\mu$m) layer of SU8 photoresist on a $75 \times 50$ mm glass plate for better adhesion of the next layers. Then we deposited the micro-grooves representing the structured roughness. We chose their height to be $\leq 0.5$ $d$ ($d$ being the mean diameter of the droplets in the emulsion), because the effect of the roughness is at that height the most pronounced [1]. As the last layer we deposited the channel walls ($H_{\text{wall}} \simeq 180$ $\mu$m). We used a $24 \times 75$ mm microscope glass slide as a cover plate on which we drilled holes for inlet and outlet prior to bonding. Using a syringe and a needle we injected small amount of Norland Optical Adhesive (NOA 63; Norland Products Inc., USA) all over the outside of the channel walls. Then on the two end of the device we put a piece of microscope cover slips ($s = 220$ $\mu$m) as a spacer, put on the cover plate with holes, fixed with a paperclip and cured the adhesive under UV light. Then the final channel height, $H$, was determined by the thickness of the spacer, i.e. $H = 220\mu$m.

**Surface modification and wetting of the channels:** We rendered the surface of the microchannels hydrophilic: the bonded microchannels were placed into plasma chamber and we applied oxygen plasma for 2x40 second. Right after plasma activation we injected 5% aqueous solution of PVP (polyvinylpyrrolidone, Sigma-Aldrich, Germany) through the channels at 1 mL/h for the period of 2 hours. This formed a stable coating on the surface which is highly hydrophilic. To quantify the hydrophilic character we mimicked the conditions of the modification process on bulk samples: SU8 resist was spin-coated on microscopic glass slide and cured according to standard photolithographic process. The SU8-cover glass along with a bare glass slide was exposed to oxygen plasma for $2 \times 40$ s, then immersed into 5% PVP solution for 2 hours under light stirring. The samples were then cleaned with distilled water, and dried. Then a drop of 2 $\mu$L of distilled water was placed on them and their contact angle measured with sessile drop technique. Also we left some SU8-covered and bare glass samples untreated and used as reference. Measured values of the PVP treated SU8-glass and bare glass were $(24 \pm 4°)$ and $(20 \pm 2°)$ respectively, while contact angles of their reference counterpart (untreated) were $(72 \pm 3°)$ and $(57 \pm 3°)$ respectively. We measured the contact angle of a water drops also after 3 months of the PVP treatment and didn't find any significant change.

**Emulsion size and size distribution:** Sample of the prepared emulsion was diluted in aqueous 1% TTAB solution. Then a few drops were placed between two microscope cover slips and a large number of images were taken under bright field optical microscope with a $100\times$ magnification objective. The images were analyzed by the software FIJI [2]. Approximately 8500 droplets were measured and averaged to determine the mean droplet diameter and the polydispersity of the emulsion. The measured values were $d = 4.75$ $\mu$m and $\text{CV} = \sigma_d/d \times 100\% = 60.1\%$. Samples of the emulsion were taken few times within a 2 months period during which the experiments took place. Moreover we measured samples before injecting the emulsion into the microchannels and after they few thought it. We didn't observe any change neither in time or due to the flowing in the microchannels.

**Rheological measurements:** A stress controlled rotational rheometer (ARES 4400, TA Instruments) with a cone-plate geometry (25 mm diameter, 0.04 radians) was used to measure the bulk rheological properties of the emulsion $\Phi = 0.875$. The flow curves were well fitted using a Herschel-Bulkley model $\sigma = \sigma_{\text{Y}} + A\dot{\gamma}^n$, with parameters $\sigma_{\text{Y}} = 55.14$ Pa, $A = 31.41$ Pa s$^{1/2}$ and $n = 0.5$.

* ladislav.derzsi@unipd.it
† matteo.pierno@unipd.it
‡ sbragaglia@roma2.infn.it

**Particle Tracking Velocimetry (PTV):** PTV was performed using a Nikon Eclipse Ti-E inverted microscope coupled with a sCMOS camera (Andor Zyla 5.5). We imaged the fluorescent tracers using a Nikon Super Plan Fluo objective with a magnification of 60×, working distance WD = 2 mm and numerical aperture NA = 0.7. By illuminating particles with a DPSS laser beam (wavelength of 522 nm, power of ≃ 50 mW) we obtained a depth of field $\delta_z = 1.5\ \mu$m $\lesssim 0.5\,d$ for each $z-$stack. As fluorescent tracers we used ThermosScientific FluoSpheres (carboxylate-modified microspheres), size of ≈ 0.2 $\mu$m, labelled with orange fluorescent dye: excitation peak at 540 nm, emission peak at 560 nm. A dichroic TRITC band-pass emission filter with the spectral bandwidth 570 − 620 nm was placed before the camera. We recorded z-stack images (400 frames per stack) with a resolution of 320 × 64 pixels and a frame rate up to 3500 fps. The stacks of images were then analyzed by FIJI [2] with a customized TrackMate plugin [3].

**Surface roughness and non-locality:** The dimensions of the patterned rough surfaces are summarized in Table S1. The height of the roughness is $h \simeq 2.3\ \mu$m, somewhat smaller than 0.5 $d$, so the effect of plastic activity is pronounced [1]. In each channel 3 different pressures were tested. Typical flow profiles at a fixed pressure are shown in Fig. S1. Slip on the smooth surface does not affect the slip on the rough surface and vice-versa. Then, at a fixed pressure drop, $v_{\text{smooth}}$ is nearly constant, only small random fluctuations are present due to fabrication imperfections. This yields the same (i.e. independent of the roughness) stress $\sigma_{\text{smooth}}$ in contact with the smooth wall. Furthermore, one has a linear stress distribution in the channel $\sigma(z) = \sigma_{\text{smooth}} + \frac{\Delta p}{L}(z + H/2)$ [4, 5]. Thus, for a fixed pressure drop, since the velocity profiles show different gradients close to the rough wall, we conclude that there exists a non-local behaviour (i.e. non uniqueness of the shear-stress relation) triggered by surface roughness [4, 5].

| $g$ ($\mu$m) | $w$ ($\mu$m) | | | |
|---|---|---|---|---|
| 15 | 8 | 15 | - | 37.5 |
| 20 | 8 | - | 20 | - |
| 37.5 | 8 | 15 | - | 37.5 |

TABLE S1. Gaps and post widths of the microgrooves used in the experiments.

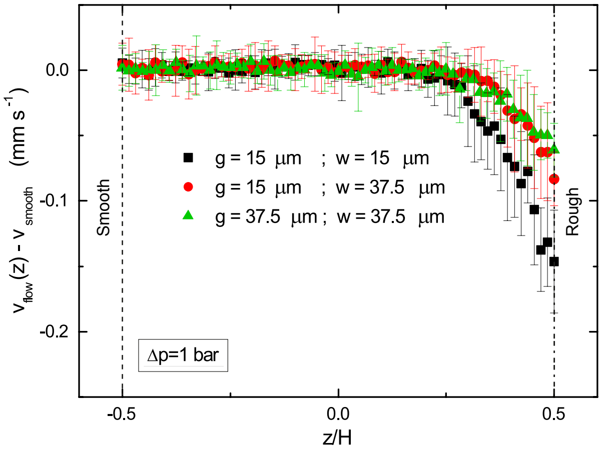


FIG. S1. Flow profiles at fixed pressure drop for different microchannels with the same $H = 220\ \mu$m.

## II. NUMERICAL SIMULATIONS

**Numerical Code:** The simulation method is based on the lattice Boltzmann methods (LBM) [6] and has been developed in the recent years by some of the authors [7–11]. They are essentially mesoscopic methods allowing the simulation of a collection of droplets above the jamming point, displaying salient features of soft-glassy materials (SGM), including yield stress [8] and non-local rheology [7–9]. For the simulations we used a new version of our CUDA implementation [12]. Since the method we use has already been described in full details in our previous papers, we refer the reader to the existing literature on the model for the relevant technical details. All our simulations are run on a small GPU [12, 13] cluster equipped with 8 nVidia Tesla K80, *i.e.* 16 K40, with 240 GB/s of bandwidth serving 12 GB of RAM per GPU [14]. The two code implementations [12, 13] allow us to collect roughly $10^4$ plastic events

every $10^6$ time steps with a total execution time of roughly 3 days for $10^7$ time steps on a system of roughly $5 \cdot 10^5$ lattice points.

**Measurement of the cooperativity length in Couette cell:** The fluidity model [4, 5, 15] describes the elasto-plastic dynamics in SGM in a mean-field spirit. The outcome of the model is a diffusion-relaxation equation for the *fluidity* field $f = \dot{\gamma}/\sigma$ (i.e. the ratio of the local shear rate $\dot{\gamma}$ and shear stress $\sigma$):

$$\xi^2 \Delta f(\vec{x}) = f(\vec{x}) - f_{\rm b}(\sigma(\vec{x})), \tag{1}$$

where $\xi$ is the cooperativity length, measuring the range of the non-local effects in the jammed material, and $f_{\rm b}(\sigma(\vec{x}))$ is the bulk fluidity, which is a function of space via the shear stress and equals the fluidity in absence of spatial heterogeneities. Equation (2) can be solved analytically in simple cases, provided that a proper boundary condition is supplied. In a steady Couette flow, in which the stress is constant, an exact calculation for a Dirichlet-type boundary condition yields

$$f(z) = f_{\rm b}(\sigma) + (f_{\rm w} - f_{\rm b}(\sigma))\, e^{(z-H/2)/\xi} \tag{2}$$

where we have assumed that the wall in $z = -H/2$ is smooth (i.e. $f(-H/2) = f_b(\sigma)$) and that $H \gg \xi$. The quantity $f_{\rm w}$ is the wall fluidity [4, 5] which parametrizes the effects of the roughness-induced fluidization. As already remarked elsewhere [5, 8], the advantage brought by the Couette cell is that the cooperativity length $\xi$ can be directly measured based on Eq. (2). The wall-to-wall distance is chosen to be $H \approx 16\,d$ and the wall at $z = -H/2$ is moved at constant velocity $u_{\rm w}$. In Fig. S2 we report representative results obtained at changing the nature of the wall in $z = +H/2$ (i.e. either smooth or rough). In presence of a smooth wall, the flow profile is essentially a linear one with a slip velocity, resulting in a rather constant fluidity throughout the channel (see right panel of Fig. S2). In presence of roughness the slip velocity is reduced and the wall fluidity increases. This produces a local viscosity (i.e. the inverse of the fluidity) that is larger close to the rough wall, and the effect spreads over a distance $\xi \approx 1.6\,d$ from the wall, in agreement with Eq. (2) (black dashed line). Above the yield stress, this value is essentially the same for all the roughness considered in the data of Fig. 4 and independent of the values of the imposed shear $u_{\rm w}/H$. Corresponding characterization of plastic rearrangements in shown in Fig. 2 of the main text and in movie M2.

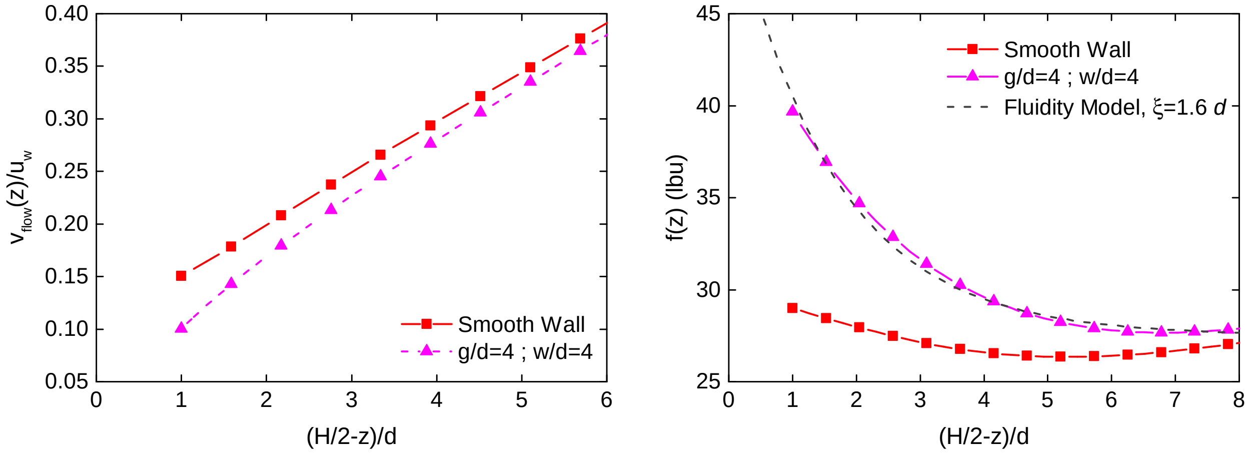


FIG. S2. Velocity and fluidity profiles in the Couette cell with smooth and rough wall.


[1] V. Mansard, L. Bocquet and A. Colin, *Soft Matter*, 2014, **10**, 6984–6989.
[2] J. Schindelin, I. Arganda-Carreras, E. Frise, V. Kaynig, M. Longair, T. Pietzsch, S. Preibisch, C. Rueden, S. Saalfeld, B. Schmid *et al.*, *Nature methods*, 2012, **9**, 676–682.
[3] J. Tinevez, N. Perry, J. Schindelin, G. M. Hoopes, G. D. Reynolds, E. Laplantine, S. Y. Bednarek, S. L. Shorte and K. W. Eliceiri, *Methods*, 2016.
[4] J. Goyon, A. Colin, G. Ovarlez, A. Ajdari and L. Bocquet, *Nature*, 2008, **454**, 84–87.
[5] J. Goyon, A. Colin, G. Ovarlez, A. Ajdari and L. Bocquet, *Soft Matter*, 2010, **6**, 2668–2678.
[6] S. Succi, *The lattice Boltzmann equation for Fluid Dynamics and Beyond*, Oxford University Press, 2001.
[7] M. Sbragaglia, R. Benzi, M. Bernaschi and S. Succi, *Soft Matter*, 2012, **8**, 10773–10782.

[8] M. Benzi, R. Sbragaglia, P. Perlekar, S. Bernaschi, M. Succi and F. Toschi, *Soft Matter*, 2014, **10**, 4615–4624.
[9] B. Dollet, A. Scagliarini and M. Sbragaglia, *Journal of Fluid Mechanics*, 2015, **766**, 556–589.
[10] A. Scagliarini, M. Lulli, M. Sbragaglia and M. Bernaschi, *Europhys. Lett.*, 2016, **114**, 64003.
[11] A. Scagliarini, M. Sbragaglia and M. Bernaschi, *Jour. Stat. Phys.*, 2015, **10**, 1–10.
[12] R. Benzi, M. Bernaschi, L. Rossi, M. Sbragaglia and S. Succi, *Phys. Rev. E*, 2009, **80**, 066707.
[13] M. Lulli, M. Bernaschi and M. Sbragaglia, *arxiv.org/abs/1607.00908*, 2016.
[14] nVidia Corporation, *Tesla GPU Literature*, `http://www.nvidia.com/object/tesla_product_literature.html`.
[15] L. Bocquet, A. Colin and A. Ajdari, *Phys. Rev. Lett.*, 2009, **103**, 036001.
